# Supplementary material for: Online Deep Clustering for Unsupervised Representation Learning
Source: arXiv:2006.10645 source file (2020-06-18)
Supplement: Supplementary file 1 [file appendix.tex]

% !TEX root = ../supp.tex

\appendix

\section{Clustering Visualization}
We visualize some representative clusters, as shown in Figure ~\ref{fig:cluster_vlz}. Apart from clusters within existing classes in ImageNet annotations, we surprisingly find that some clusters explore new classes and object relations beyond ImageNet annotations.
The phenomenon reveals the possibility of unsupervised learning to capture new semantics beyond manual annotations.

\if 0
\begin{figure*}[h]
	\centering
	\includegraphics[width=\linewidth]{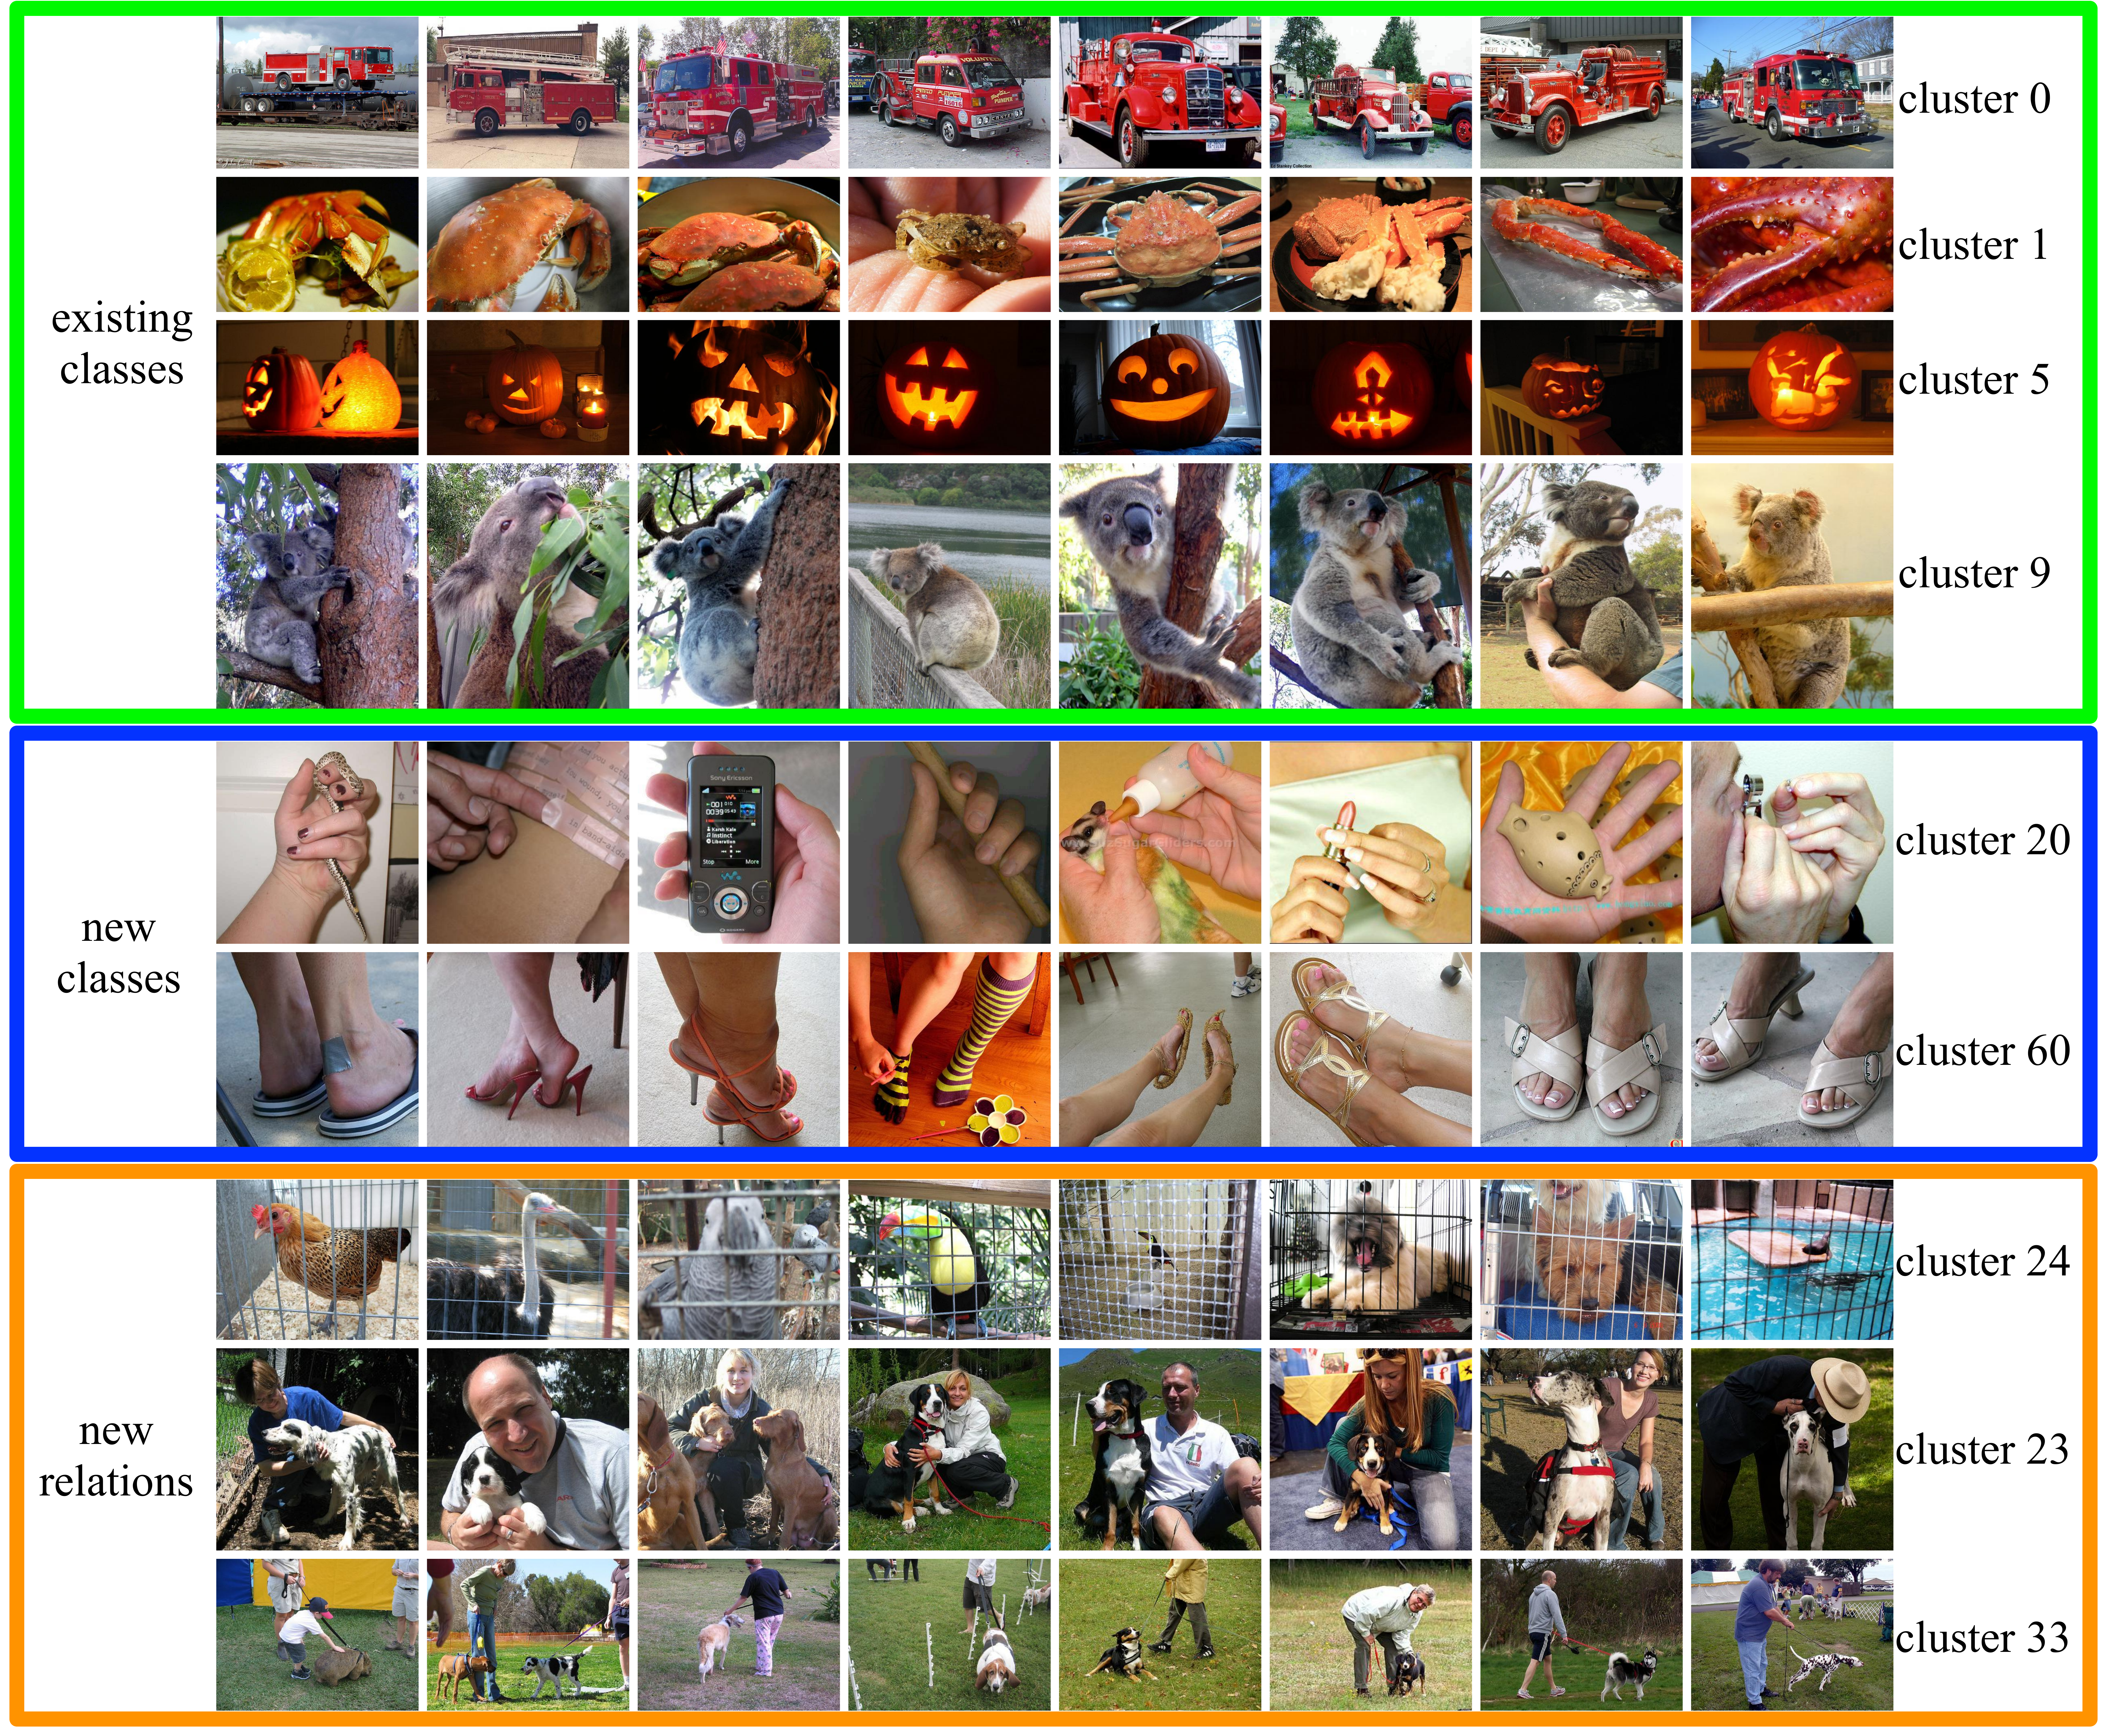}
	\caption{This figure shows part of selected clusters. Each row represents a cluster. The semantics of most clusters are within existing classes in ImageNet annotations, shown in the green box. We also find some new semantics discovered by ODC, shown in the blue box. For example, the two rows in the blue box group ``hand'' and ``feet'' respectively, while ``hand'' or ``feat'' is not a category in ImageNet annotations. ODC also potentially group images with similar relations between objects. As shown in the orange box, the clusters represent ``animal in cage'', ``person holds dog'' and ``person leads dog with a rope'' respectively.}
	\label{fig:cluster_vlz}
\end{figure*}
\fi
